# Supplementary material for: Hyper-VolTran: Fast and Generalizable One-Shot Image to 3D Object Structure via HyperNetworks
Source: arXiv:2312.16218 source file (2024-01-05)
Supplement: Supplementary file 1 [file supp.tex]

% \clearpage
% \setcounter{page}{1}
% \maketitle

In the main manuscript, we have provided the pipeline of our work and the 
In this supplementary material, we provide the details of our method, settings, and additional results.

\begin{figure}[t]
    \centering
    \includegraphics[width=.48\textwidth]{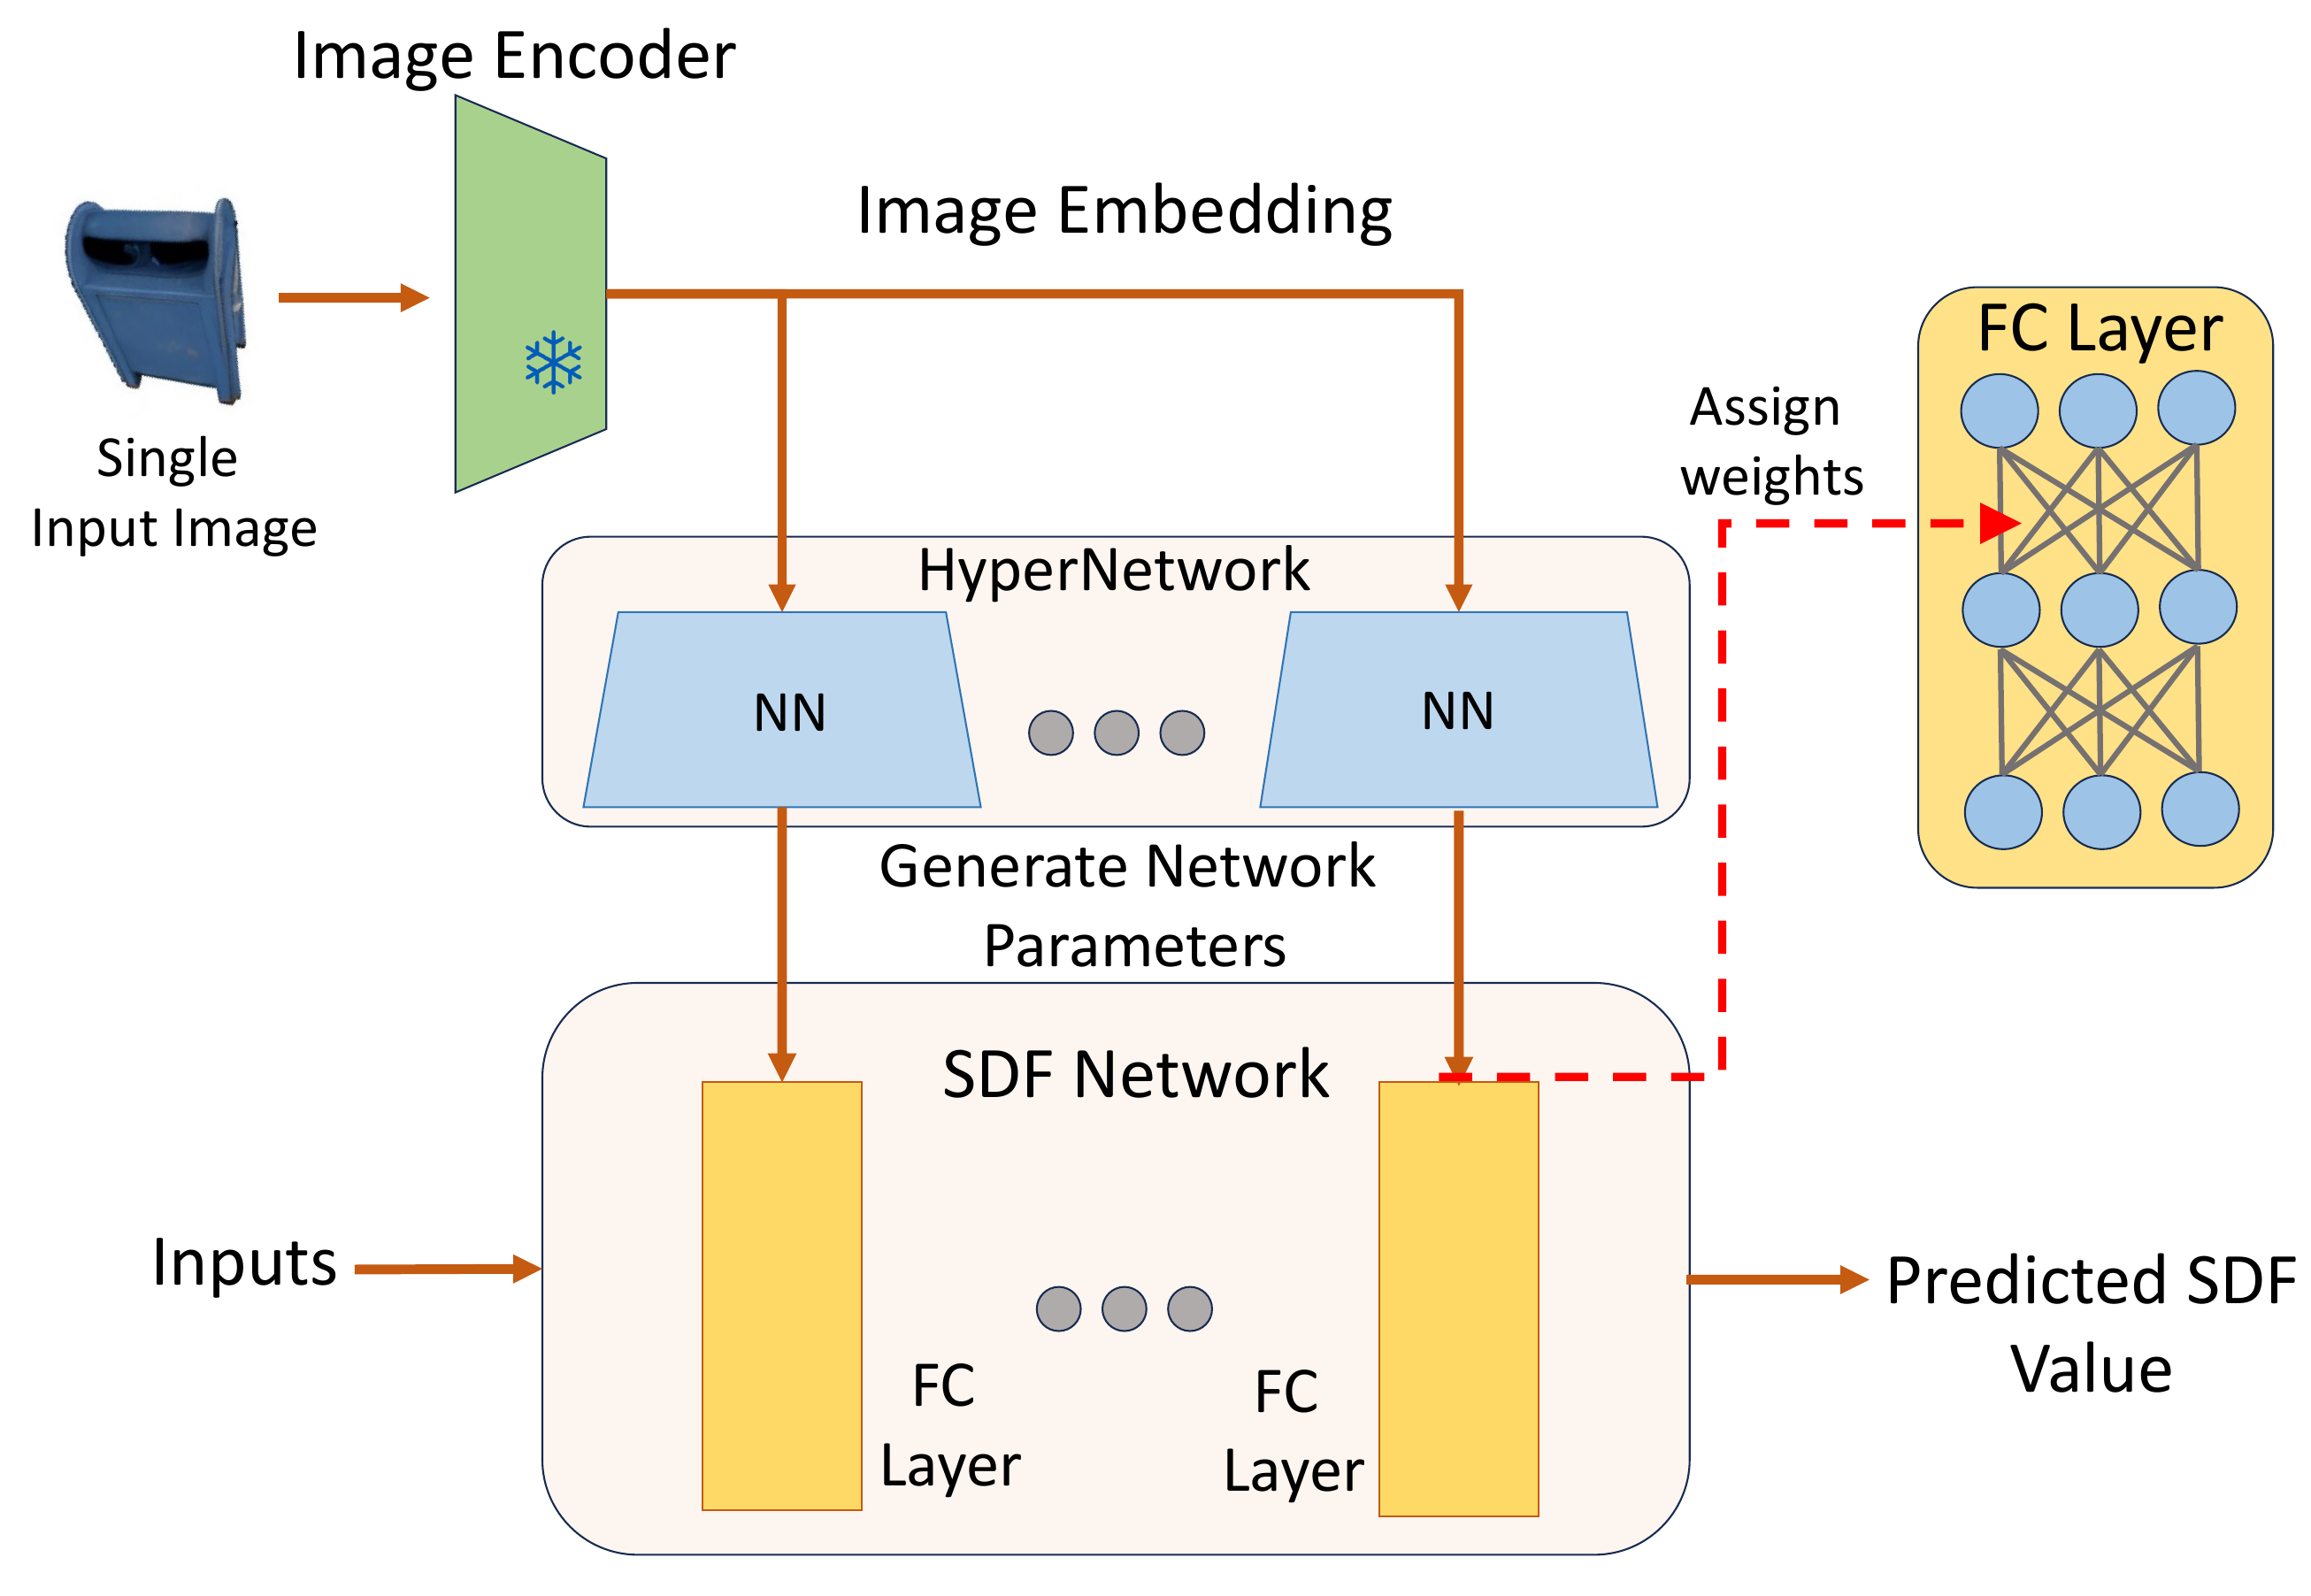}
    \caption{The detail of our HyperNetwork architecture to assign weights to the SDF network. The input is obtained from the image embedding of an image encoder.
}
\label{fig:hypernet_module}
\end{figure}

\begin{figure}[t]
    \centering
    \includegraphics[width=.48\textwidth]{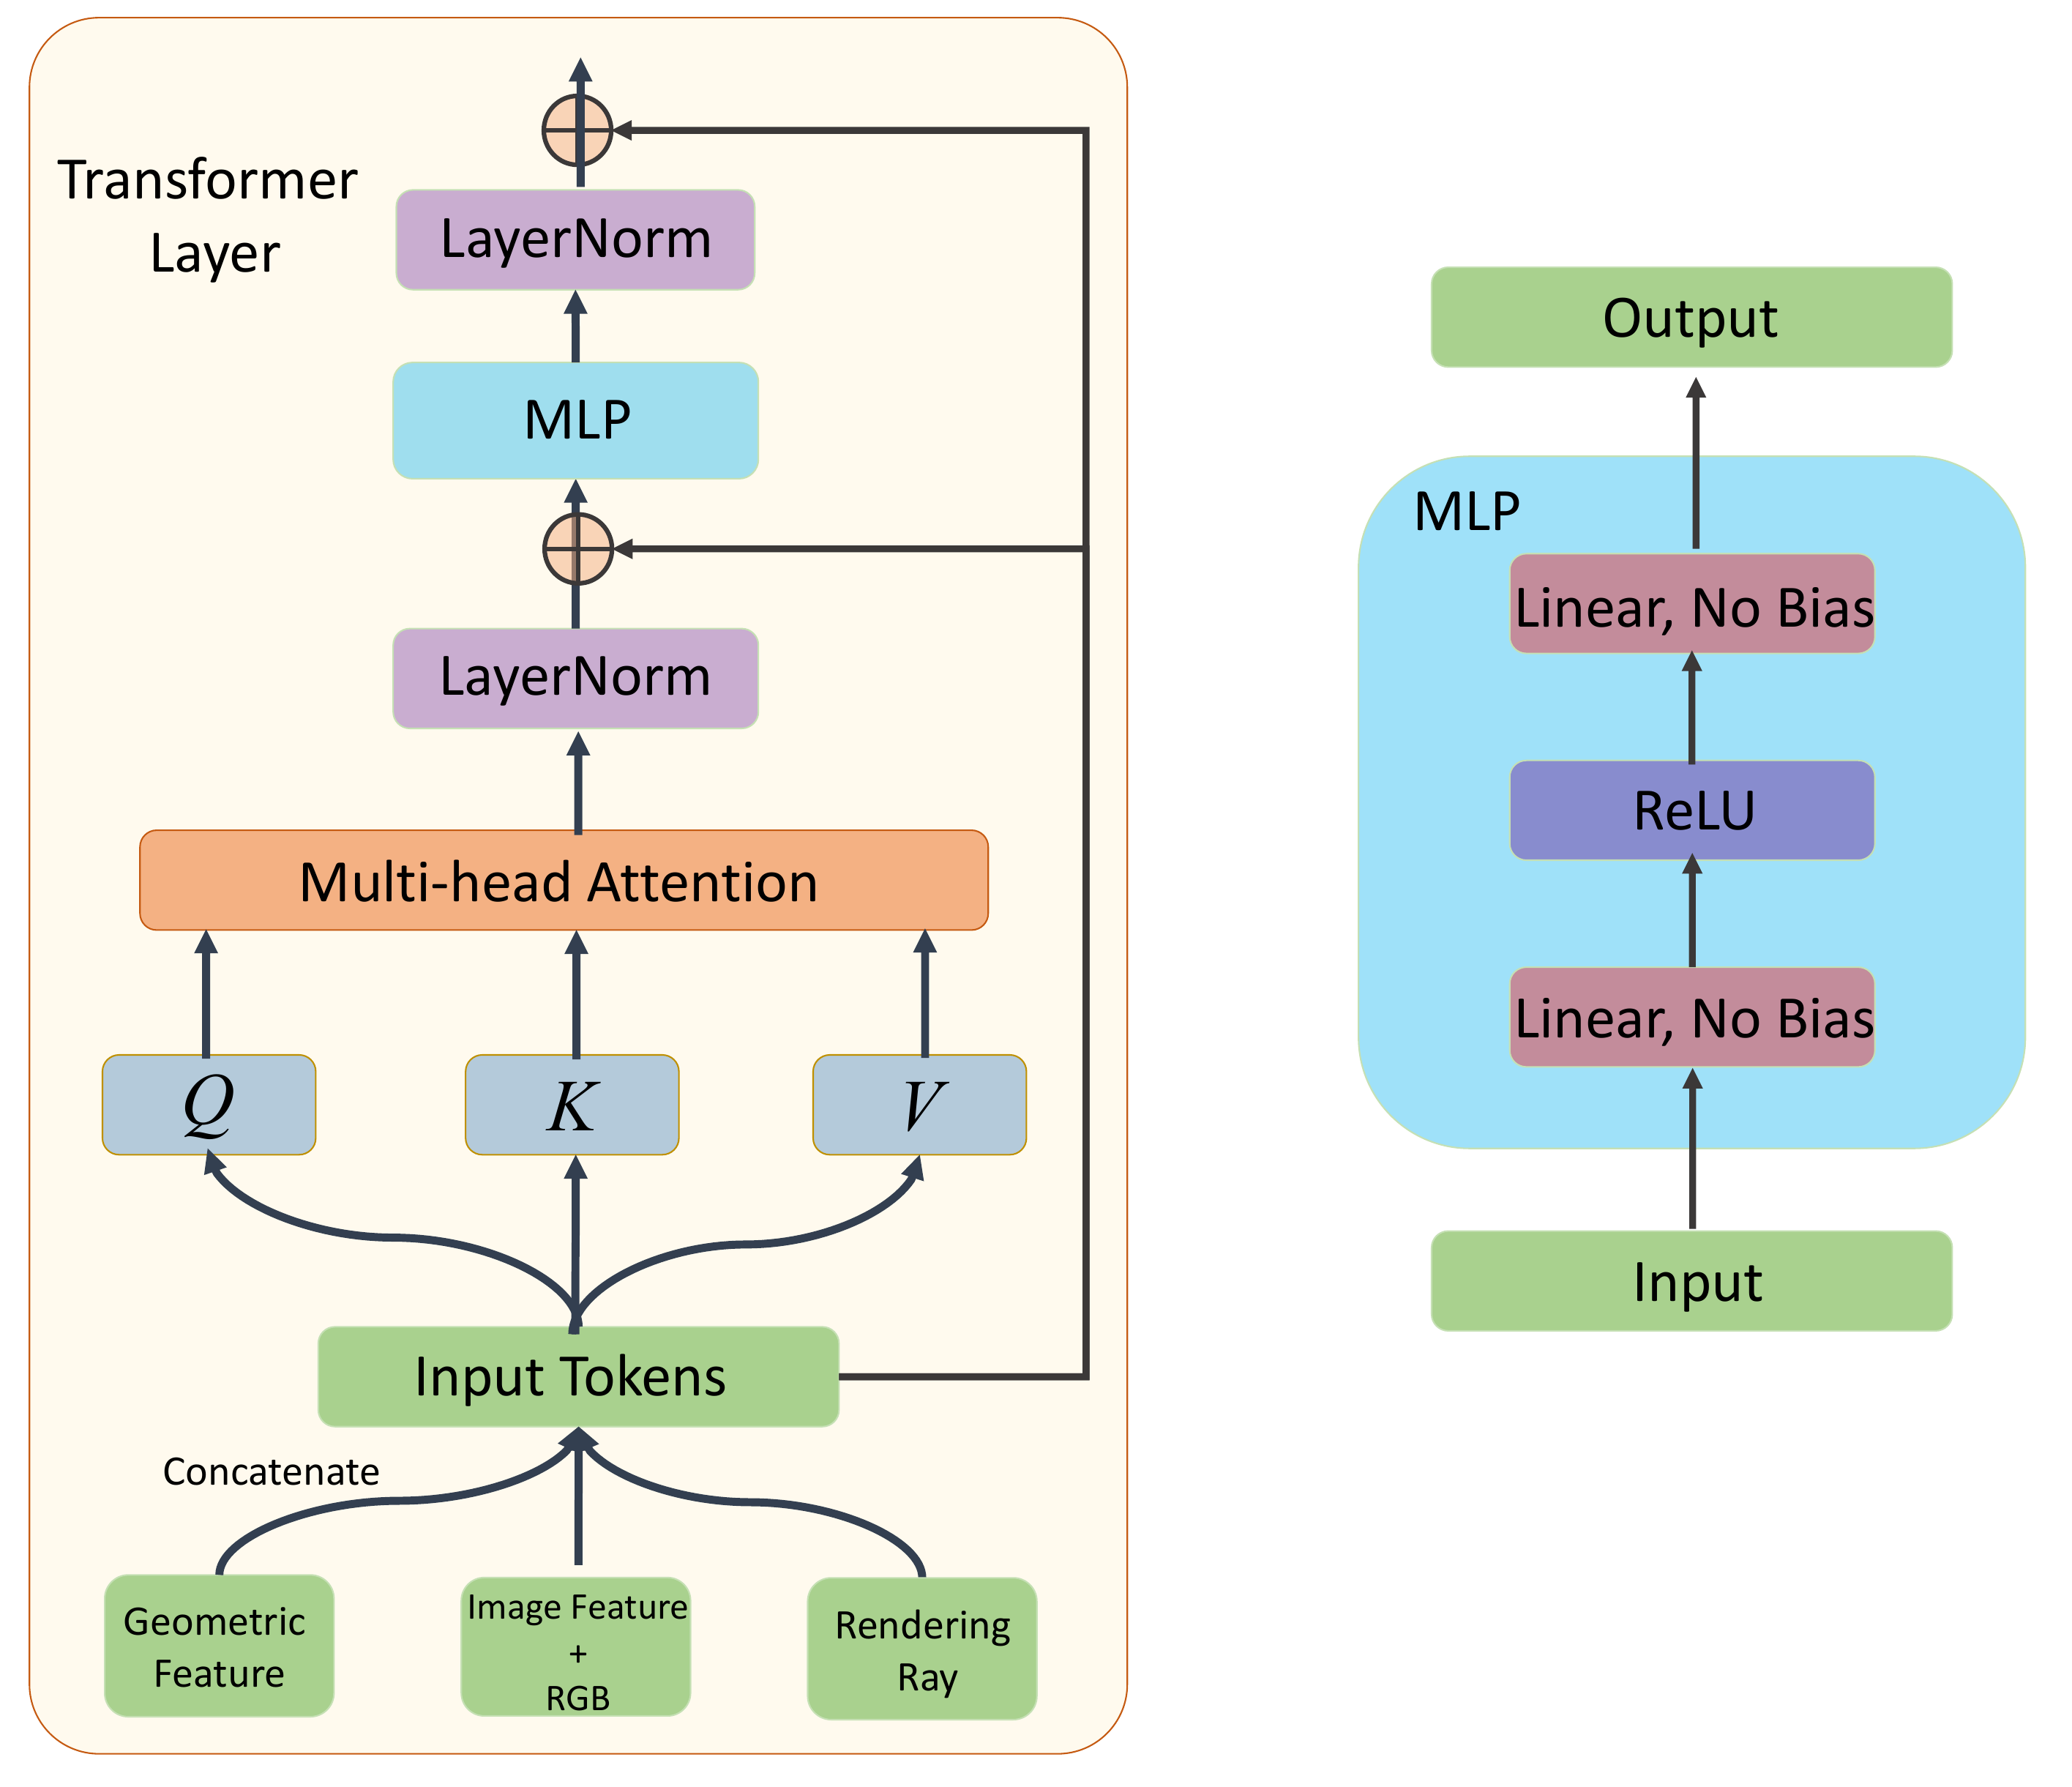}
    \caption{The detail of our Volume Transformer \textbf{VolTran} architecture as an aggregator from the features of multiple views.
}
\label{fig:transformer_module}
\vspace{-0.3cm}
\end{figure}

\section{Details of Our Proposed Modules}
\label{sec:modules}
In the main paper, %\textsection~\ref{sec:proposed_method}, 
we mentioned two modules constructing our framework to improve both generalization and consistency. We would detail out these two modules namely HyperNetworks and Voltran in the following sections.
\subsection{HyperNetworks}
The HyperNetworks~\cite{ha16hypernet} are used in our pipeline to build the SDF network. In each HyperNetwork module for each SDF network layer, we build 3 fully-connected layers with ReLU activations in the intermediate layers. In the first layer, we map from the output dimension of the text embedding which is 768 to 32 as the dimension of the hidden layer.  The input to the HyperNetwork is the image embedding as an output of an image encoder (\eg, CLIP~\cite{radford2021clip}). Please see Fig.~\ref{fig:hypernet_module} for an illustration of our method.

\subsection{VolTran: Multi-View Transformer}
The transformer module in our framework is used as an aggregator to reduce the noise impacts in multi-view synthesized images. The transformer module is fed with input tokens from the feature of each view. Fig.~\ref{fig:transformer_module} shows the detail of each component in the transformer module in VolTran. We set the multi-head number to 5 and 2 layers of the transformer with self-attention.

\begin{figure}[t]
    \centering
    \includegraphics[width=.46\textwidth]{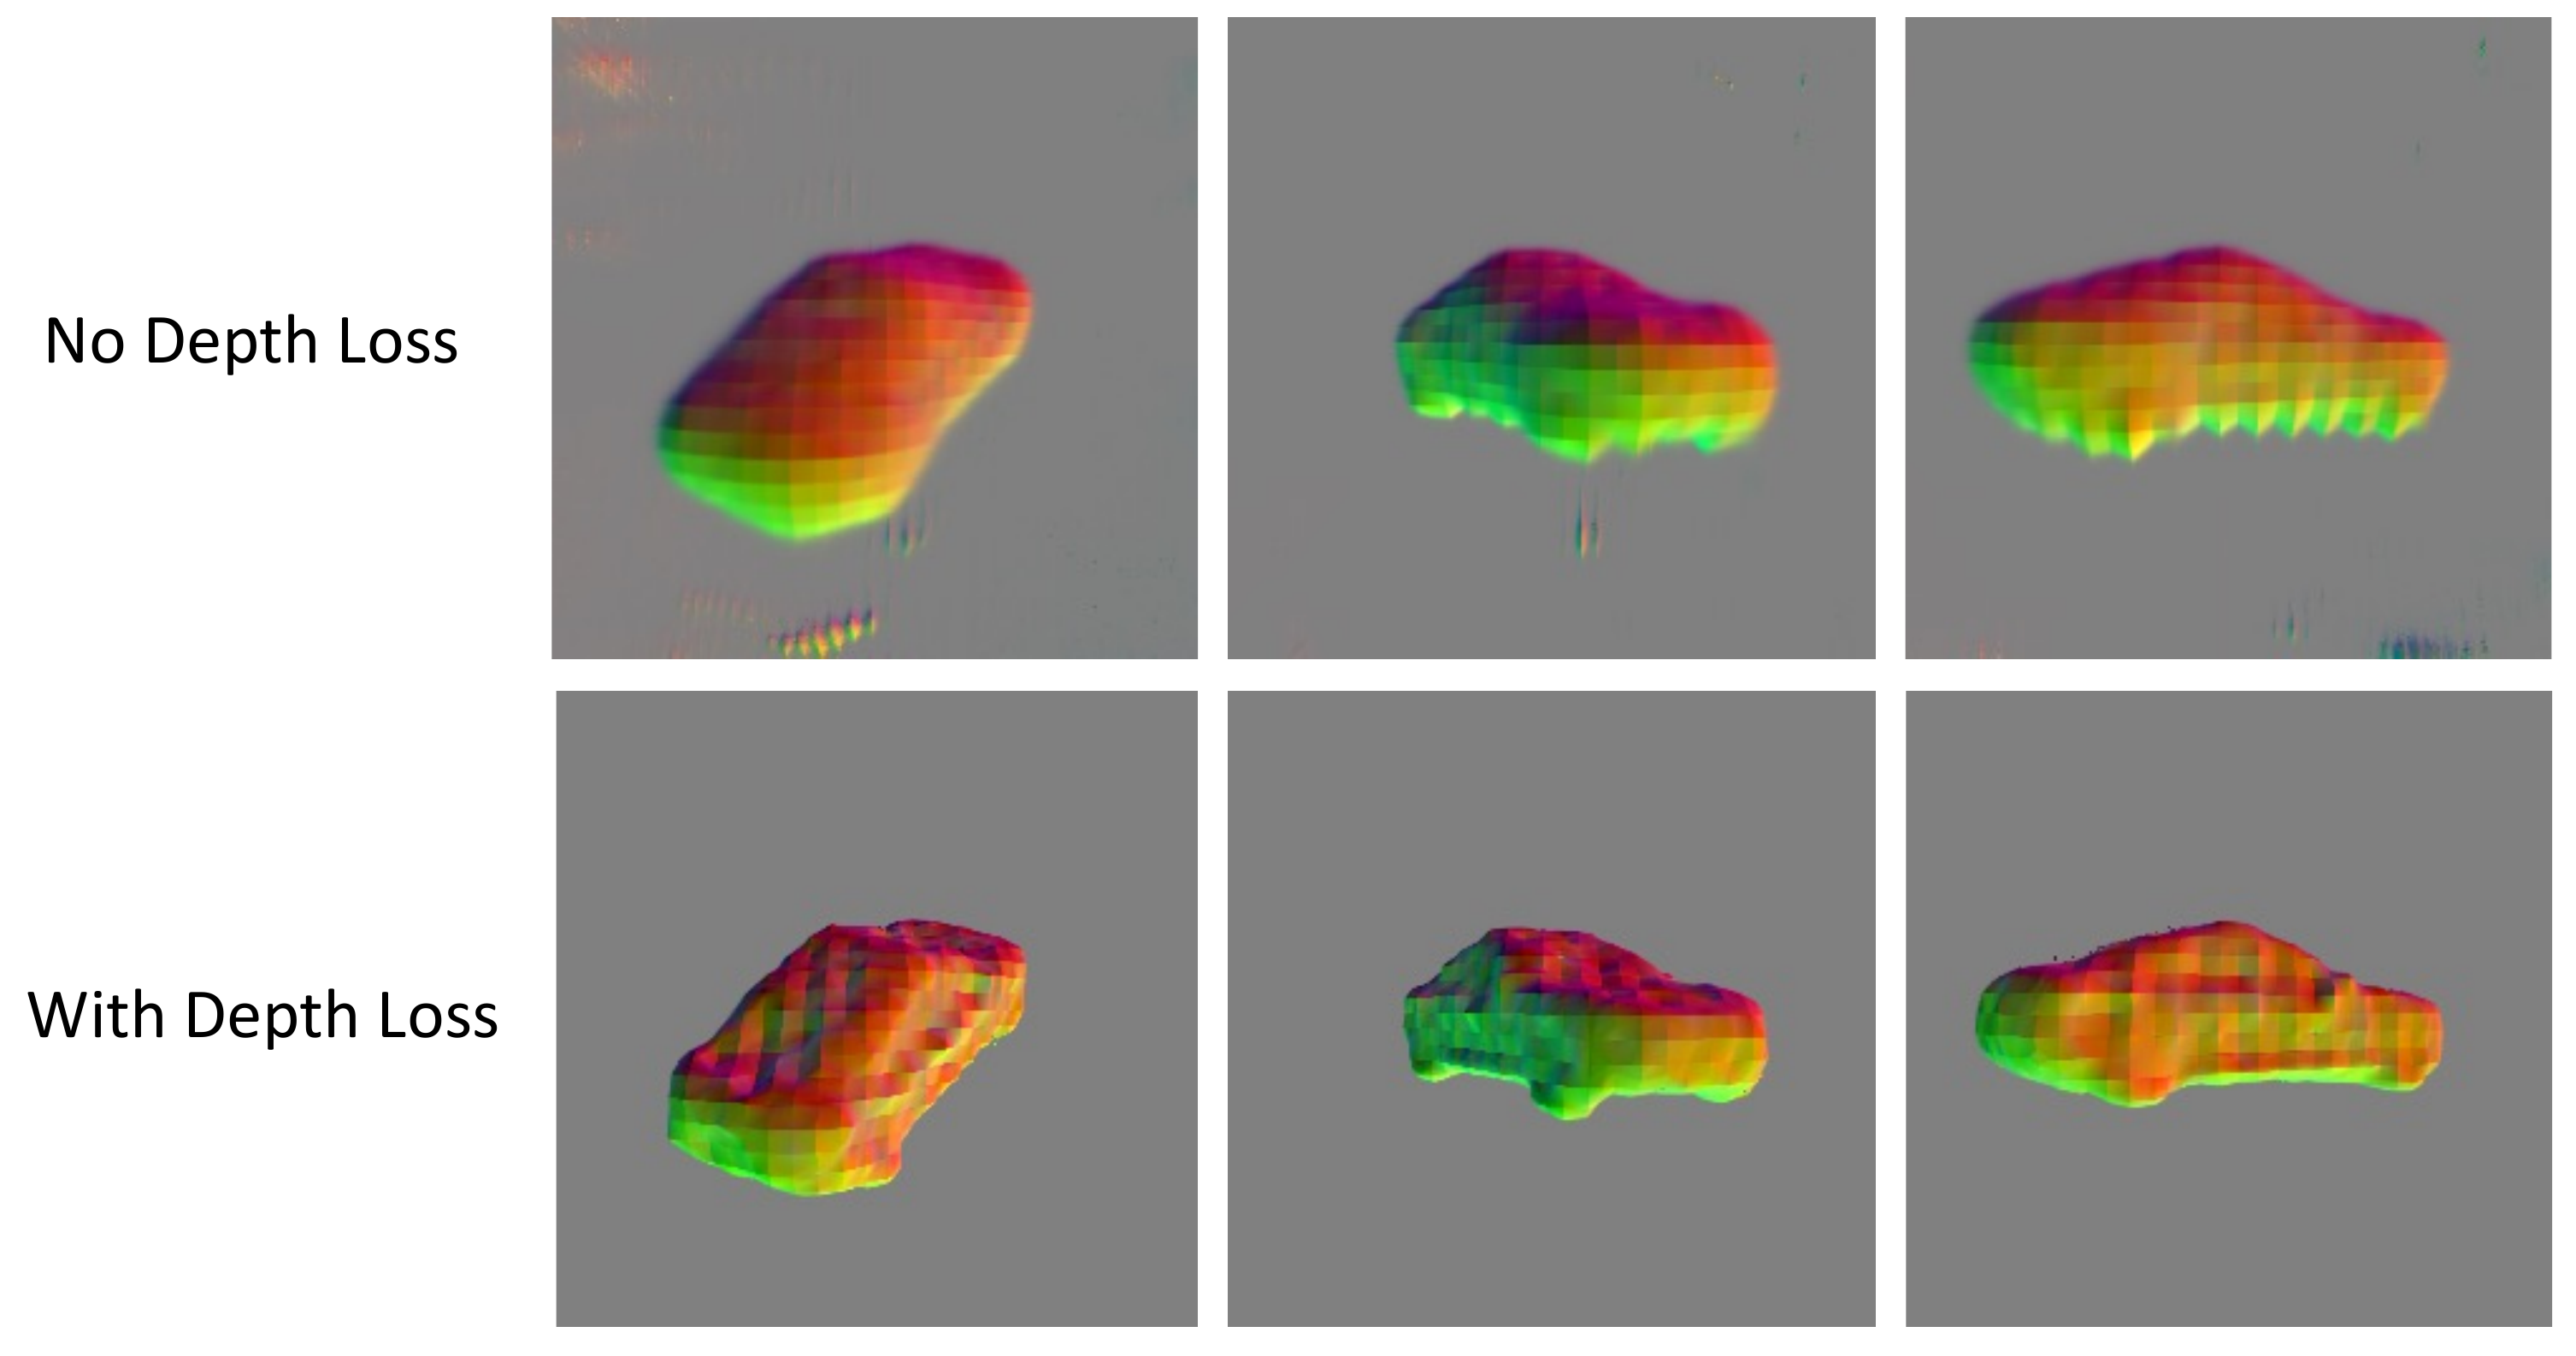}
    \caption{Comparison of including the depth loss and without the depth loss in the training stage. Without the depth loss, the shape becomes more rough and less detailed. The generated 3D scene has some residuals outside the boundaries of the shape. 
}
\label{fig:depth_loss}
\vspace{-0.2cm}
\end{figure}

\begin{figure}[t]
    \centering
    \includegraphics[width=.46\textwidth]{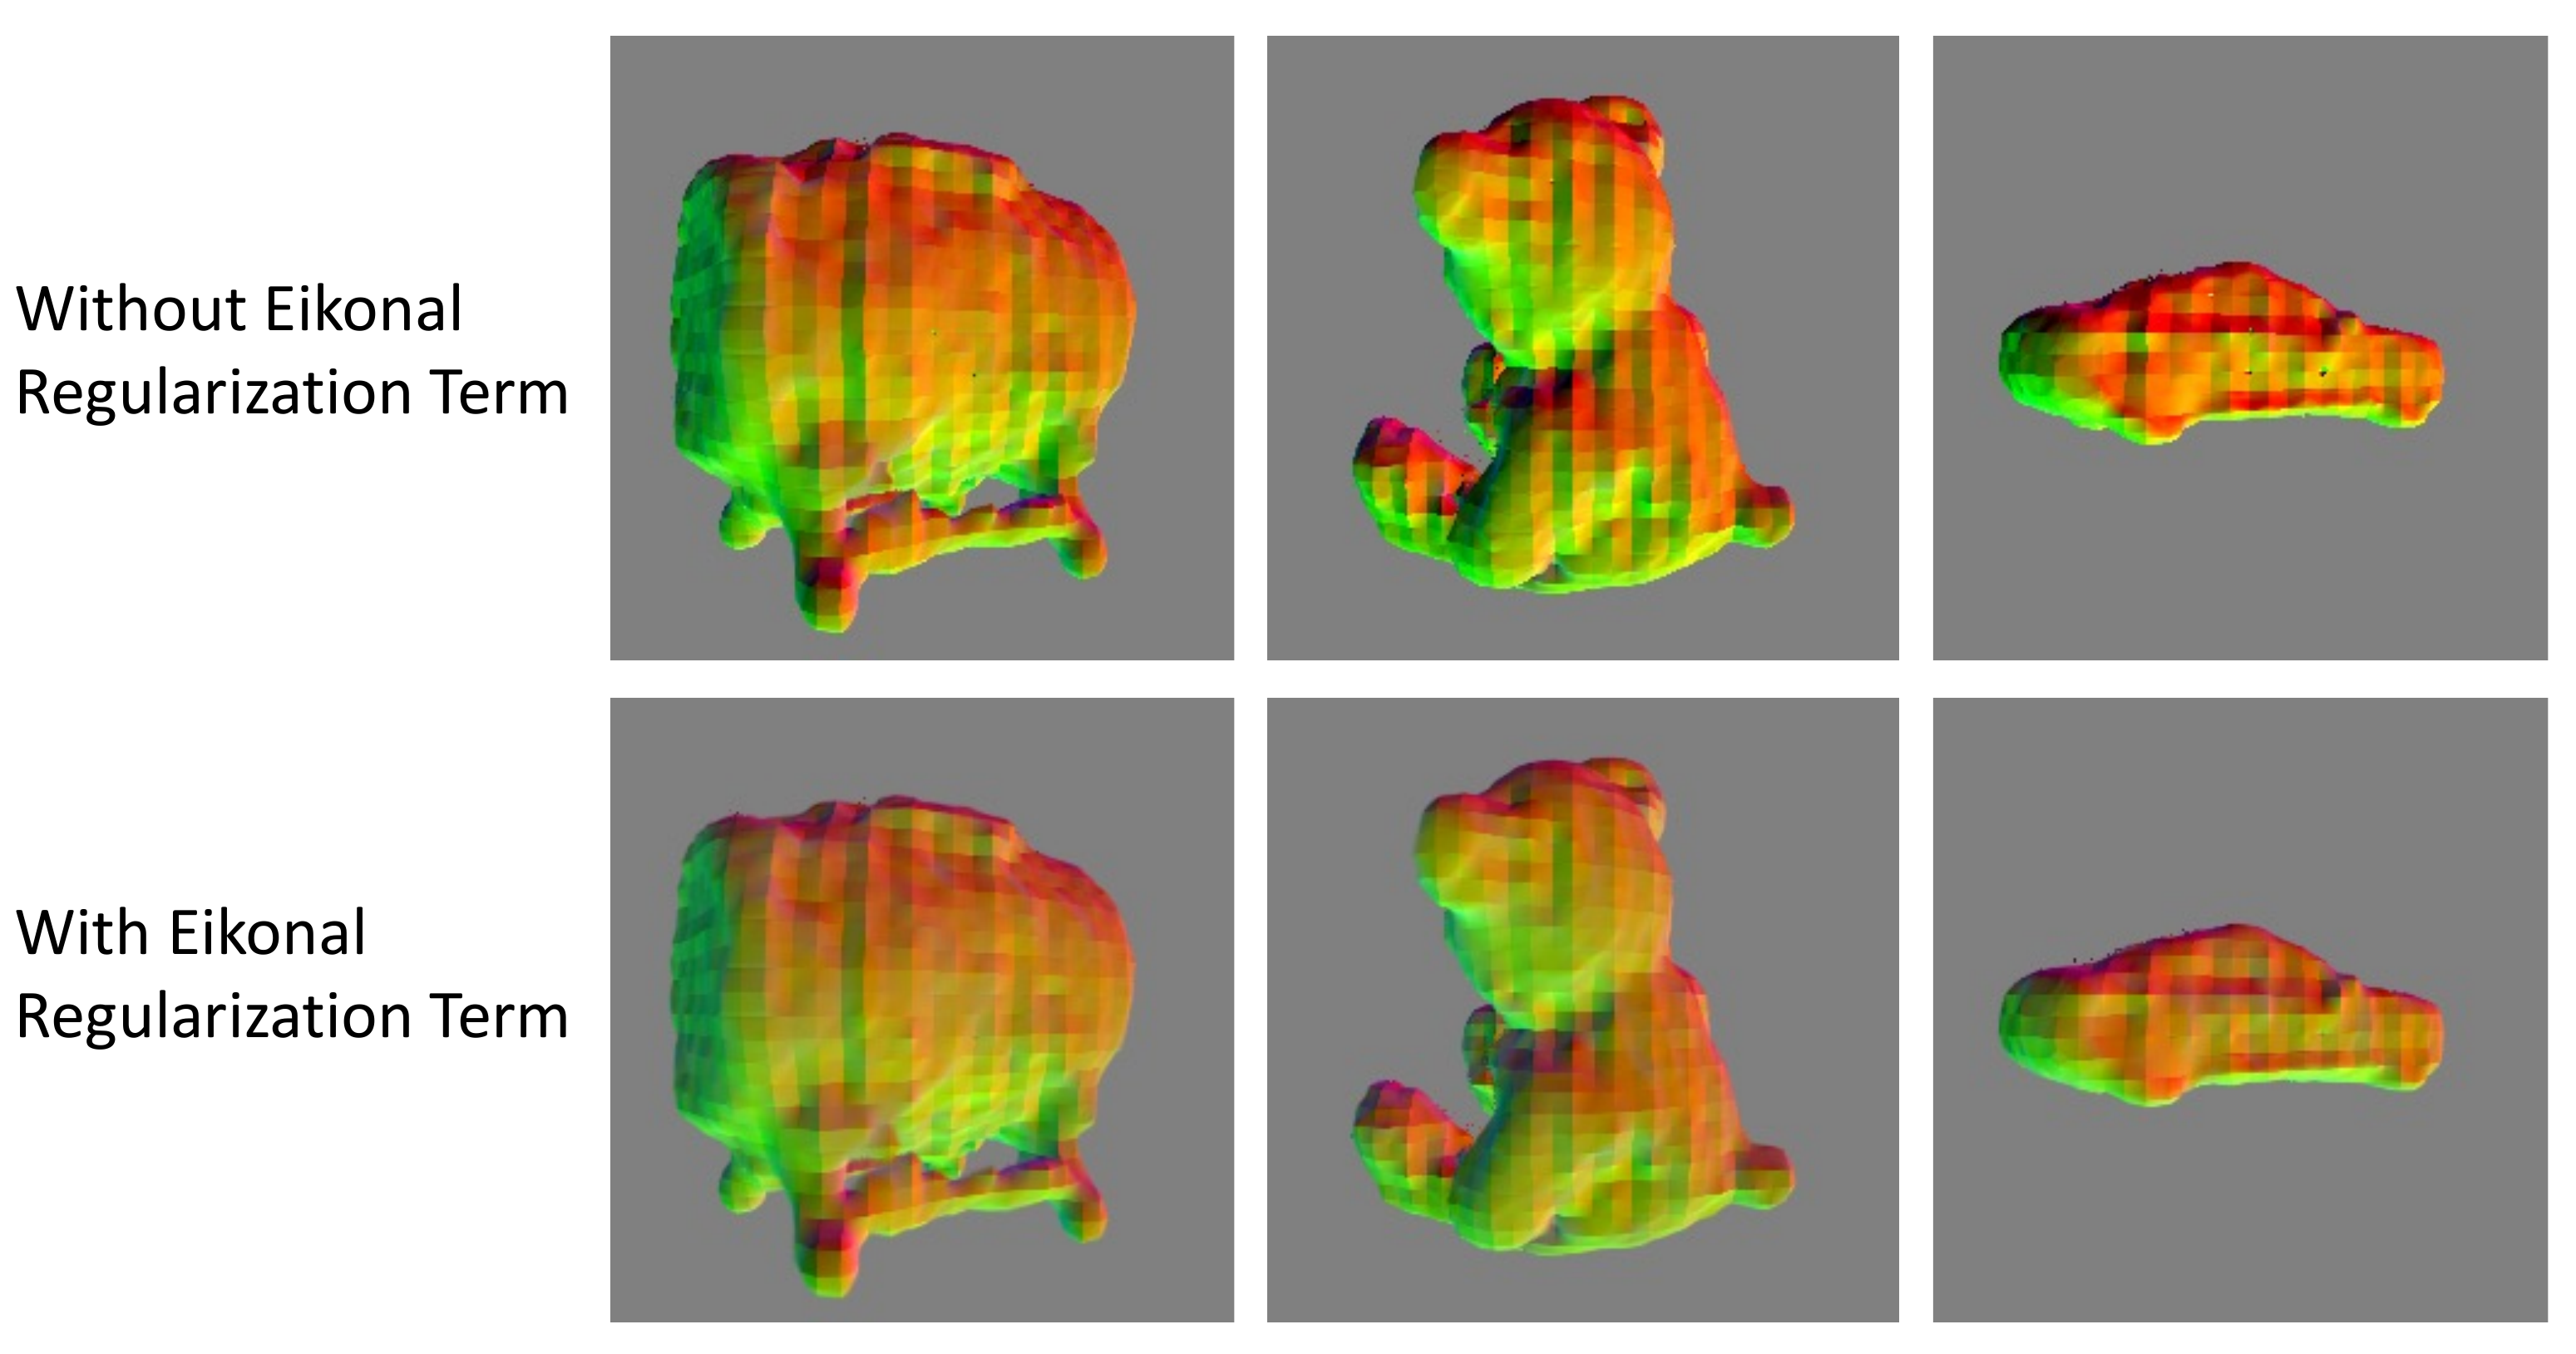}
    \caption{Comparison of including the Eikonal regularization term for smoothness in the training stage. We can observe that the upper part has very rough surface (see the high contrast between dark and bright regions of the surface) and less smooth compared to the below one trained using the Eikonal regularization term. 
}
\label{fig:eikonal_term}
\vspace{-0.2cm}
\end{figure}

\begin{figure}[!h]
    \centering
    \includegraphics[width=.46\textwidth]{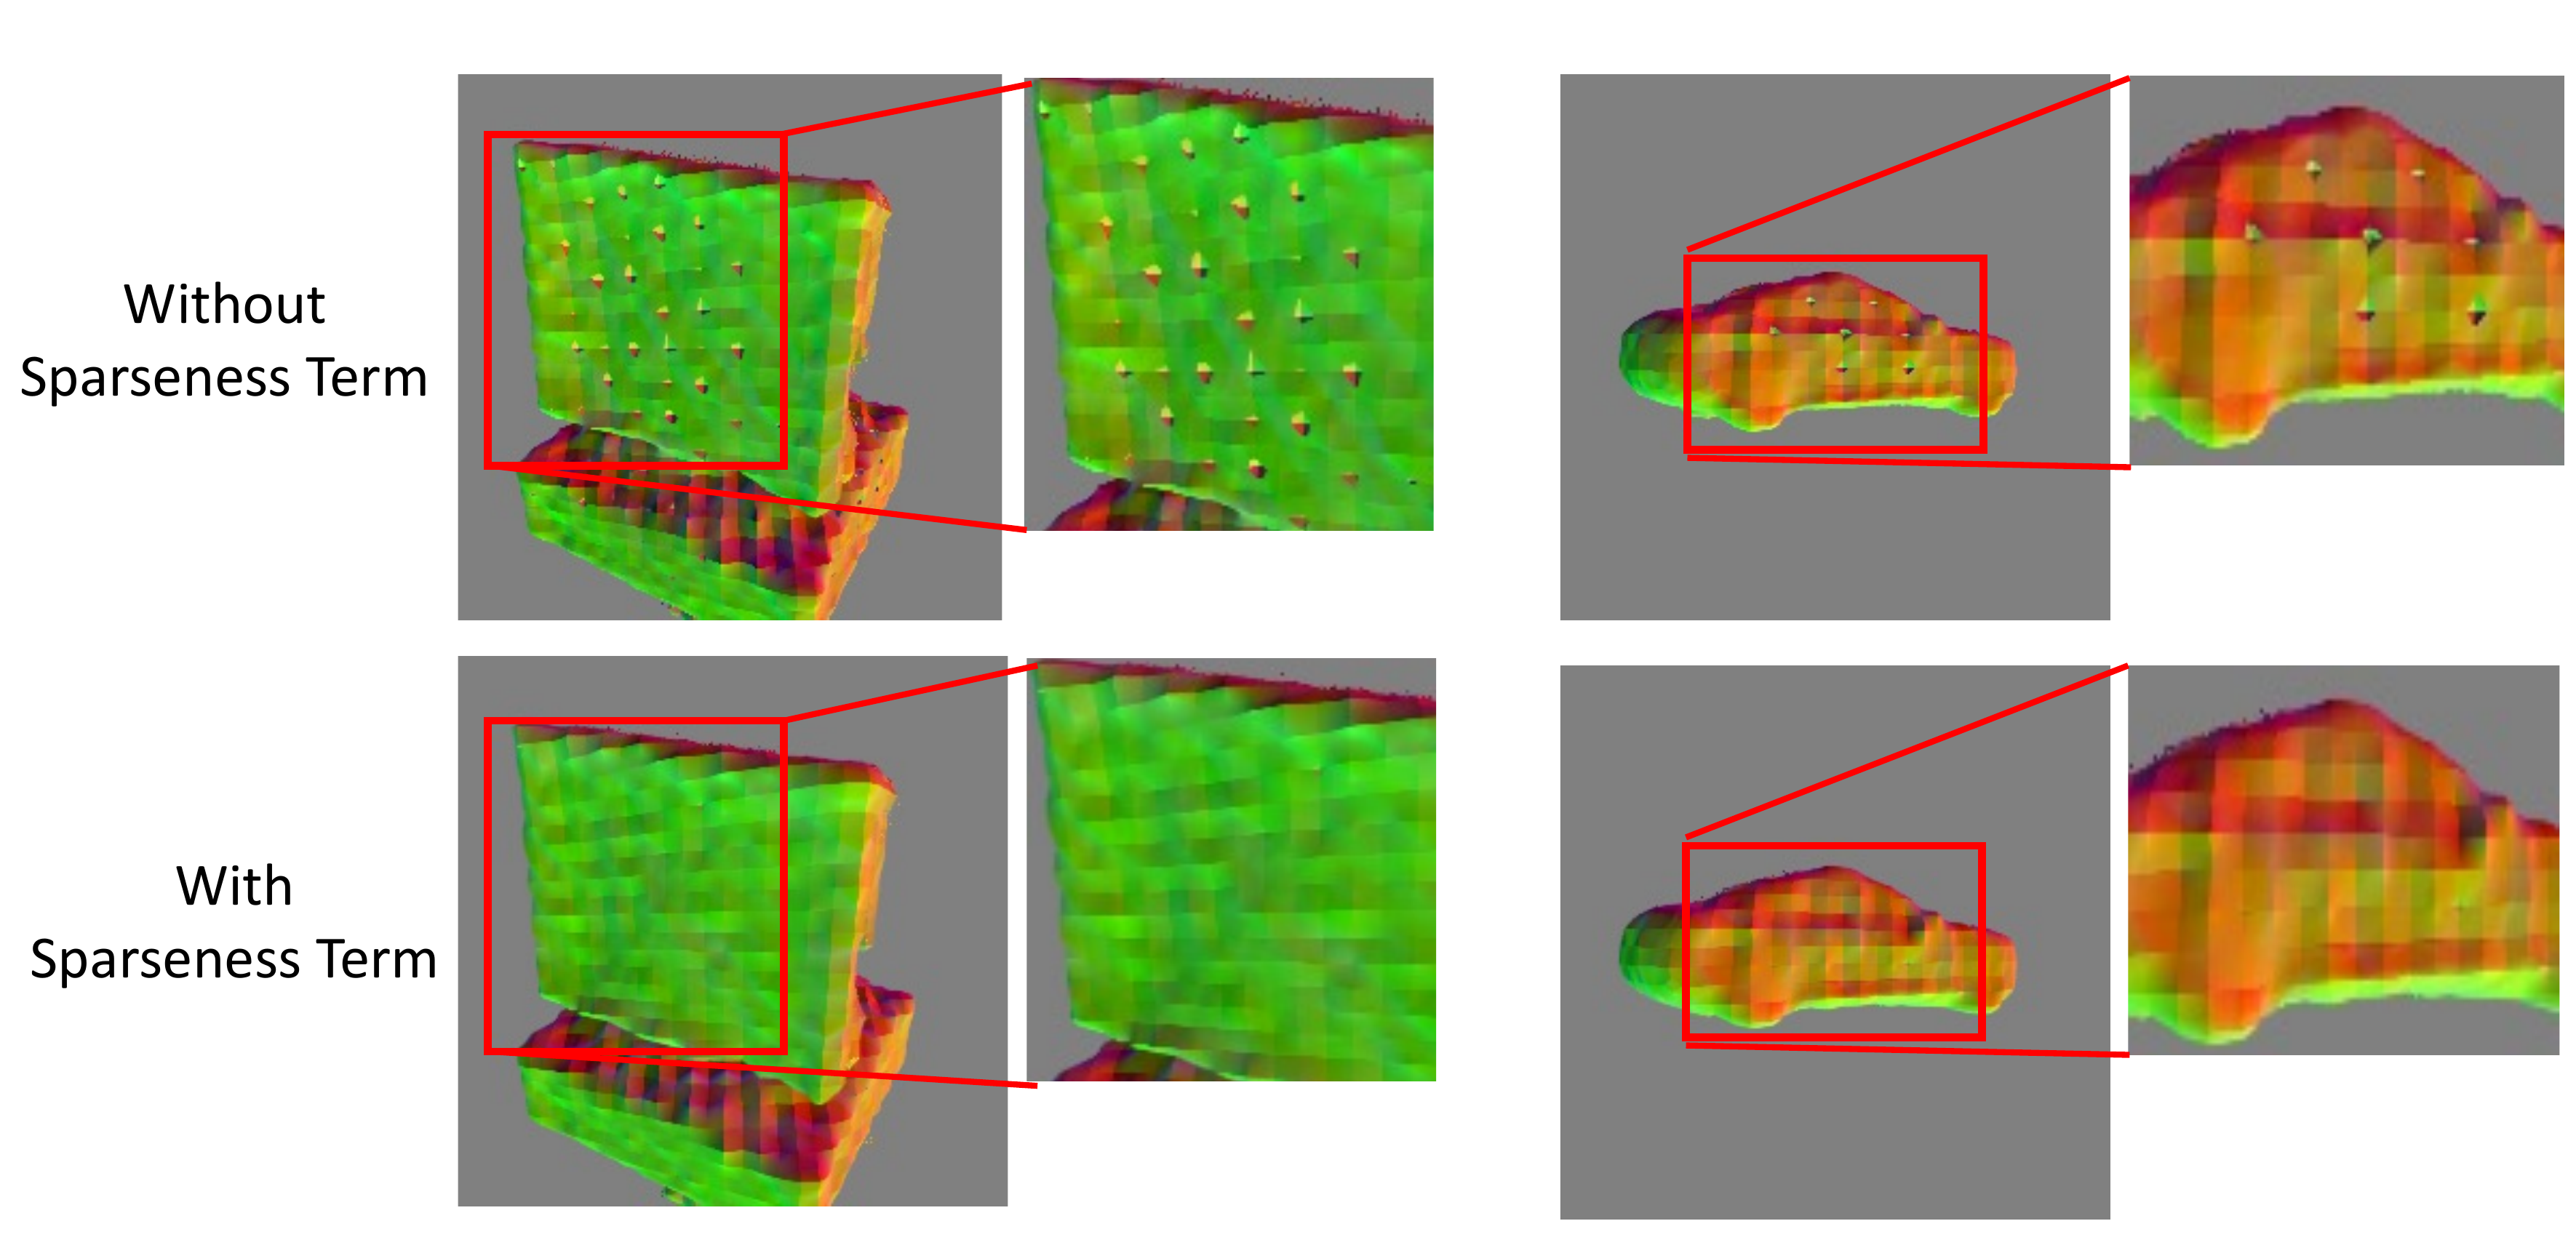}
    % \vspace{-1.4cm}
    \caption{Comparison of including the sparseness regularization term for compactness in the training stage. We  observe that the generated surface has some defects (\ie, holes) compared to the below one trained using the sparseness regularization term. 
}
\label{fig:sparseness_term}
\vspace{-0.2cm}
\end{figure}

\begin{figure*}[t]
    \centering
    \includegraphics[width=.99\textwidth]{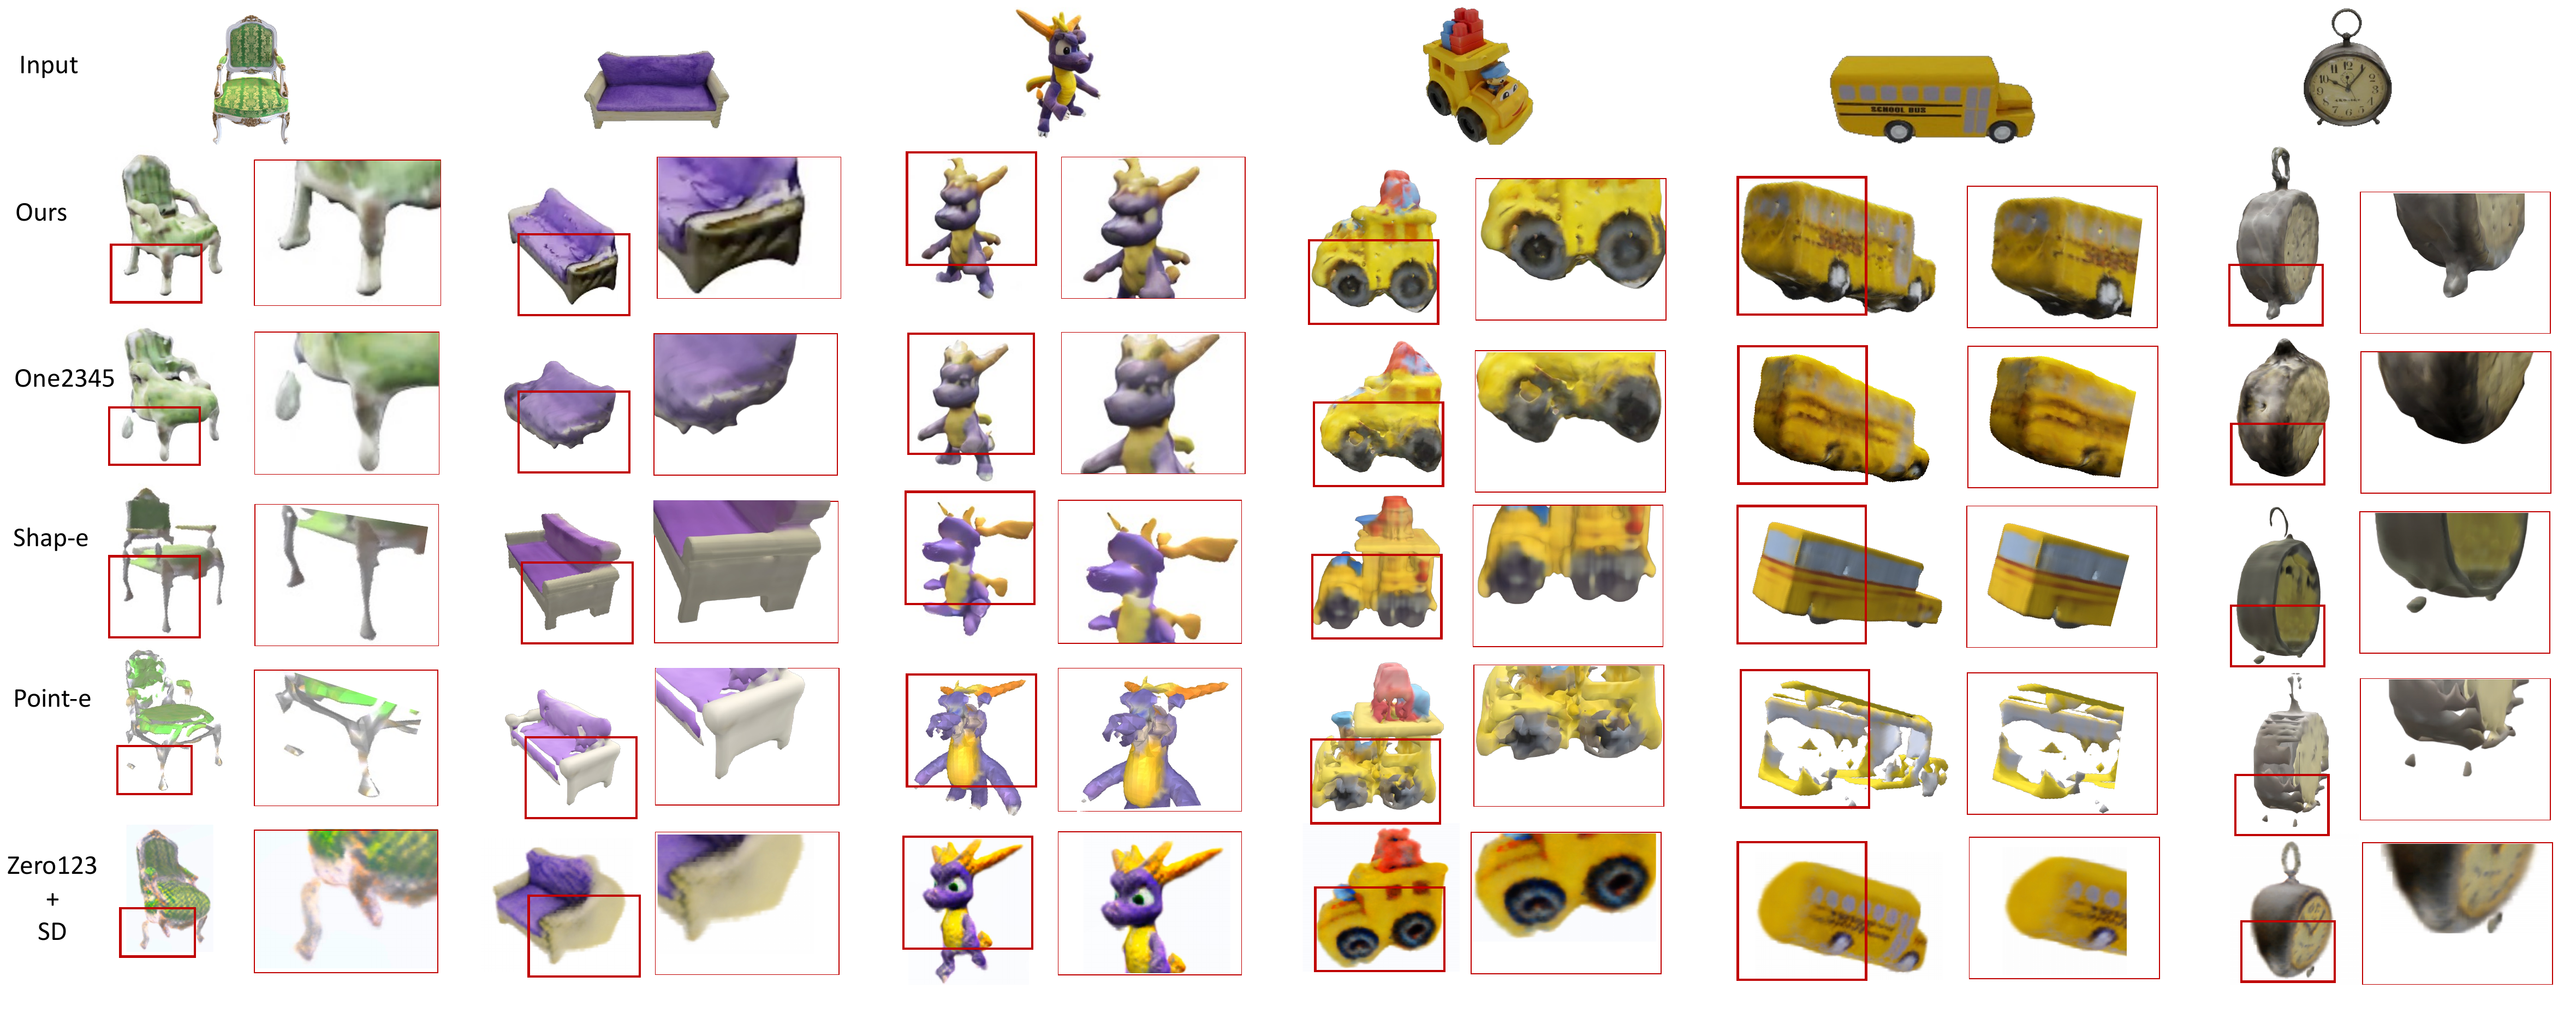}
    \caption{Comparison of our proposed method \textbf{Hyper-VolTran} against baselines with zoomed patches.  
}
\label{fig:zoomed}
\end{figure*}

% \subsection{Text-to-3D}

% \subsection{Image-to-3D Comparison with Zoomed Details}

\begin{figure*}[t]
    \centering
    \includegraphics[width=.99\textwidth]{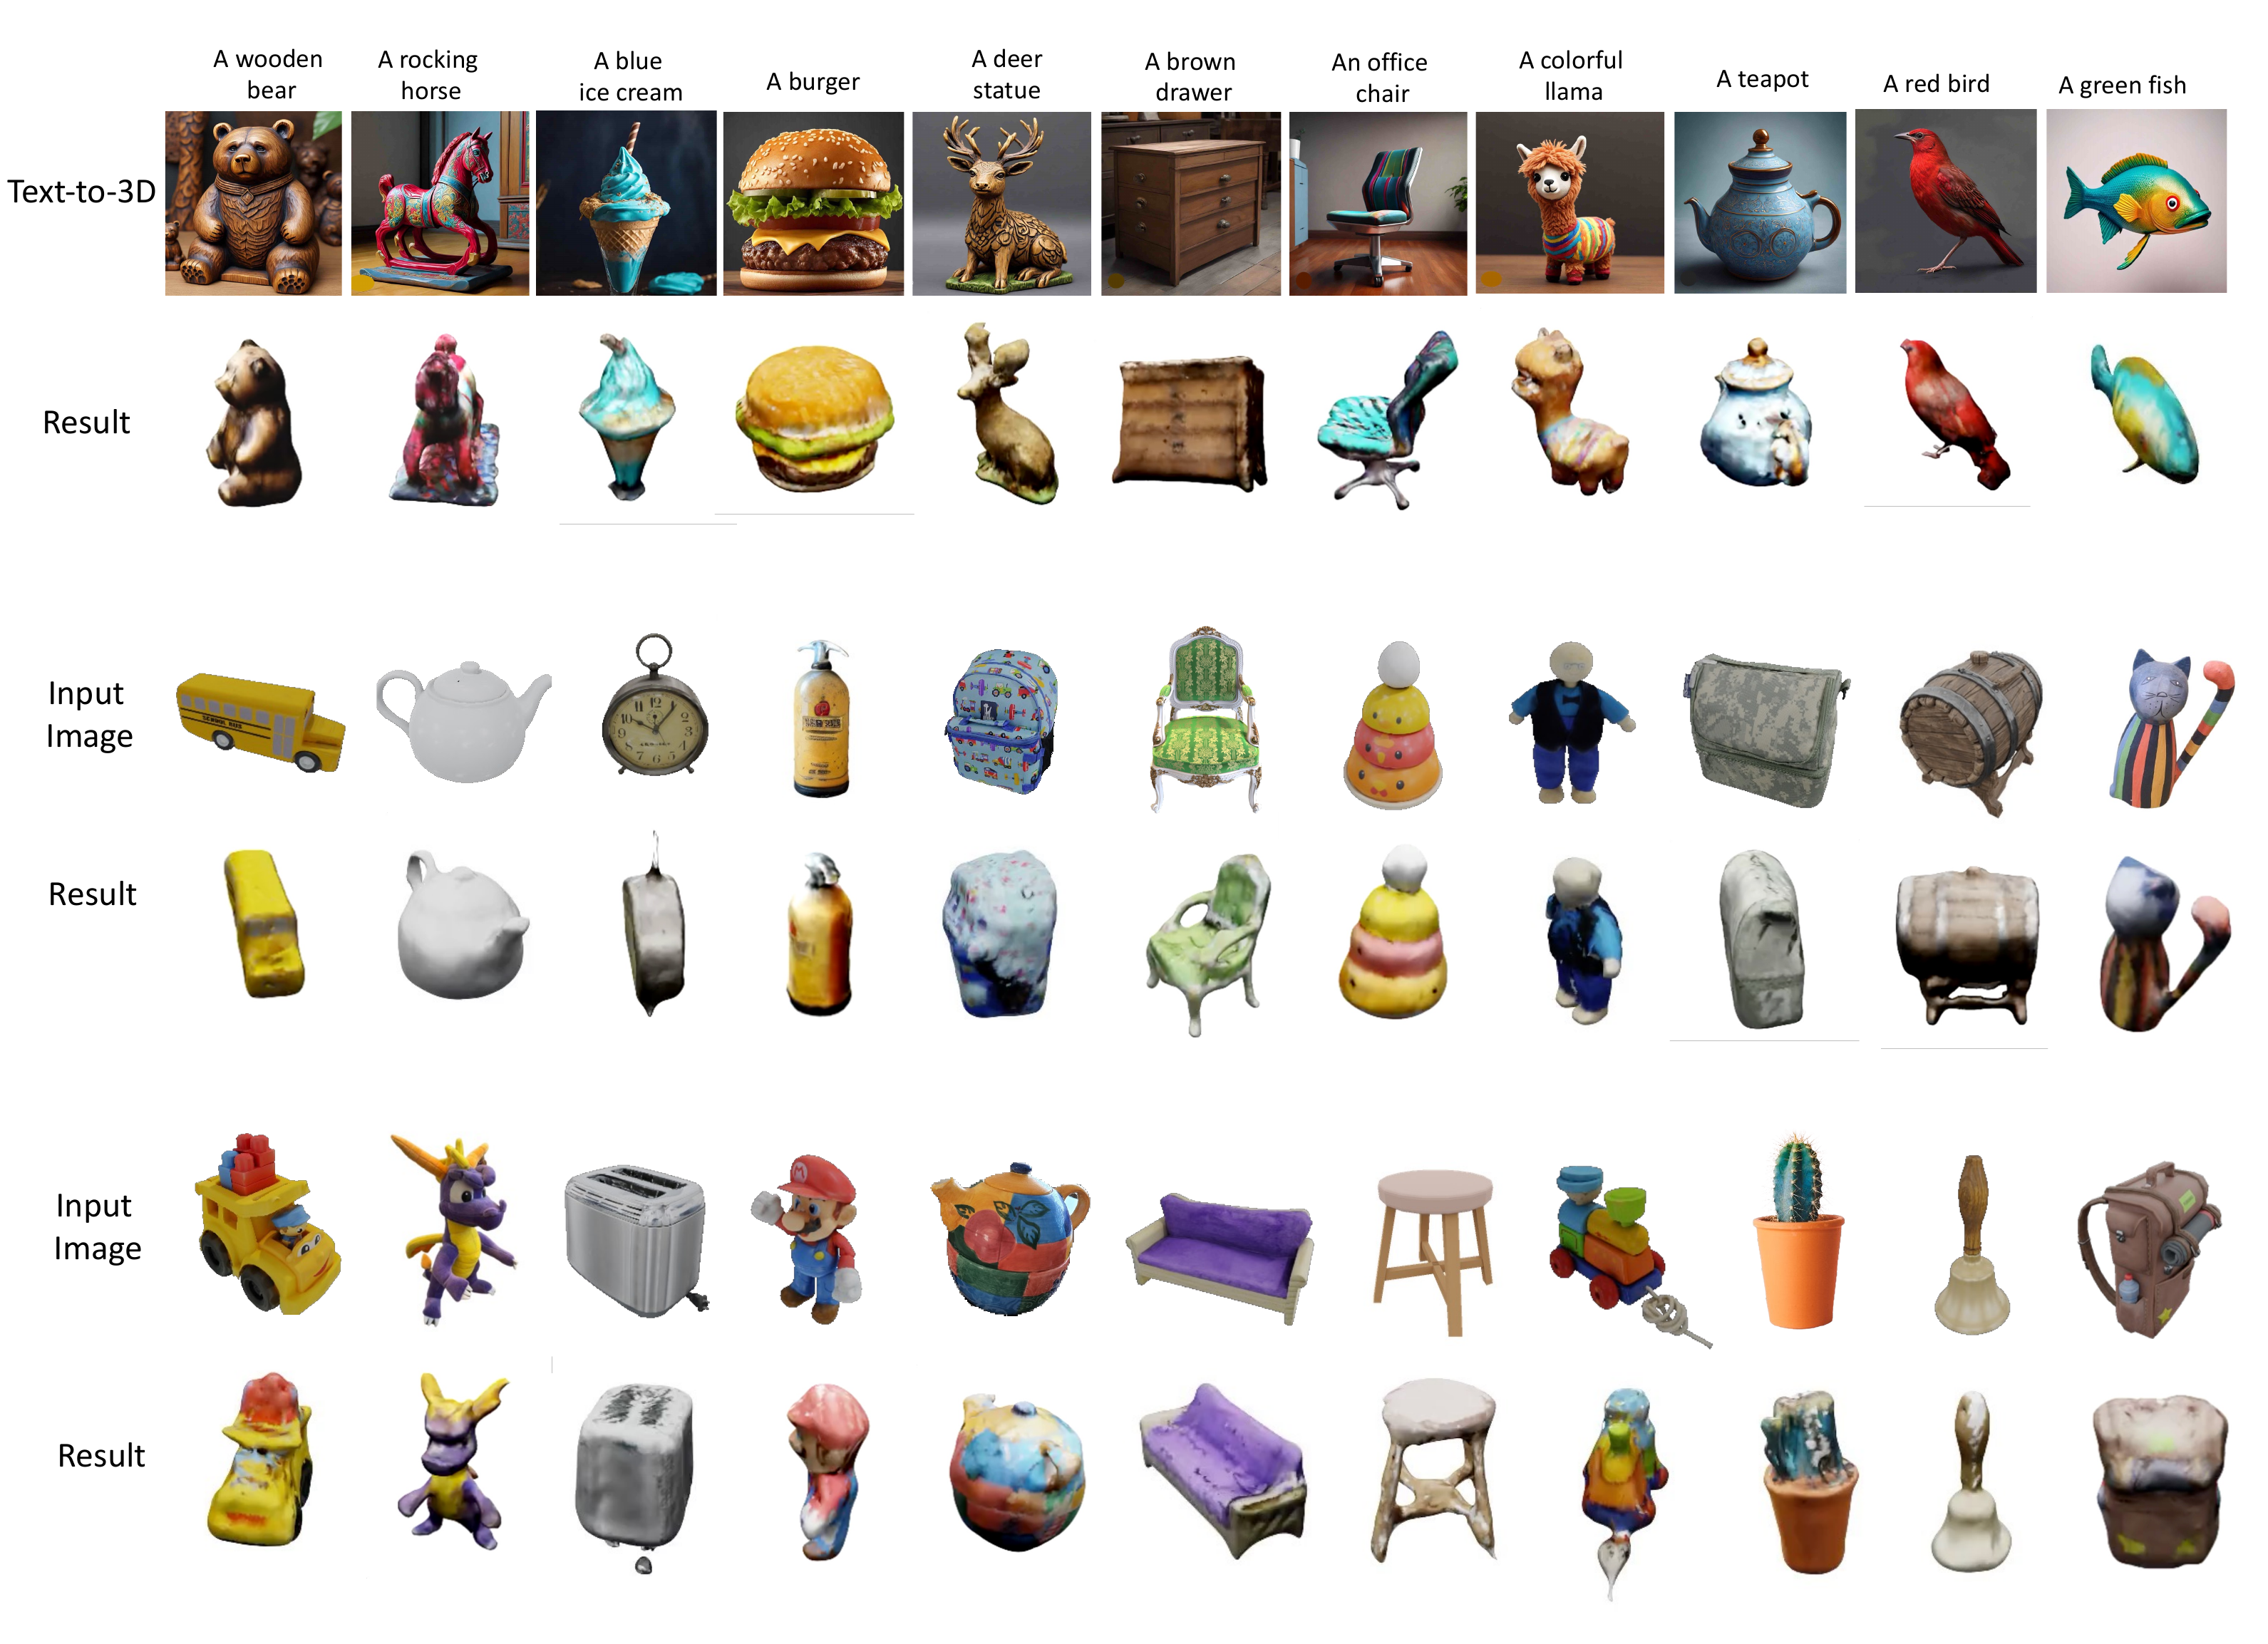}
    \caption{The results of generated 3D objects using our proposed method on text-to-3d and image-to-3d tasks.  
}
\label{fig:all_results}
\end{figure*}

\section{Ablation on the Loss Terms}
We investigate the role of each loss function to produce high-quality images. We observe that without sparseness reguralization term as described in the main paper %Equation~\eqref{eq:sparse_loss} 
impacting the capability in generating compact surfaces.  As shown in Fig.~\ref{fig:sparseness_term}, some object surfaces have some defects and impact compactness of the surface because of the uncontrollable free surfaces when we remove the sparseness regularization term.  For the Eikonal term, it is applied to regularize the SDFs and the network to have the unit $l_2$ norm gradient yielding smooth surfaces. We experimented to train the network without the Eikonal term, as a result, Fig.~\ref{fig:eikonal_term} shows that the objects have very rough surfaces due to unregularized SDFs. We also observe that the shape details of an object might not be accurately predicted without the depth loss. We also notice that the depth loss enriches the shape of an object to add more details and remove some unwanted residuals as shown in Fig.~\ref{fig:depth_loss}.

\section{Implementation and Evaluation Details}

\subsection{Hyperparameters}
In our experiments, we use 32 images as the optimal number of generated images from the outputs of a generative model. For training the model, we set the learning rate to 5e-4 and adjust it using the Cosine learning schedule. The model is trained for 300K iterations. We set the sparseness term, Eikonal term, and depth term to 0.02, 0.1, 1.0, respectively. The background ratio is set to 0.3.   
% sdf_igr_weight = 0.1
%   sdf_sparse_weight = 0.02
%   sdf_decay_param = 100
%   fg_bg_weight = 0.1
%   bg_ratio = 0.3  camera pose to be known as provided in the dataset.  

\subsection{Data Used for Evaluation}
We opt to use two datasets for our evaluation. The first dataset is obtained from 15 images proposed in RealFusion~\cite{melaskyriazi2023realfusion}, intended for evaluating rendering quality. For the GSO dataset~\cite{downs2022gso}, we pick 25 images from different categories as follows: Alarm,
Backpack, 
Bell,
Blocks,
Chicken,
Cream,
Elephant,
Grandfather, Grandmother,
Leather,
Lion,
Lunchbag,
Mario,
Oil,
Schoolbus1,
schoolbus2,
Shoeblack,
Soap,
Sofa,
Sortingboard,
Stacking cups,
Teapot,
Toaster,
Train,
Turtle.

\section{Additional Results}
\label{sec:additional_results}
In this section, we provide some more detailed images and more results in addition to the results provided in the main paper. We provide a zoomed version of the generated results in comparison to baselines in Fig.~\ref{fig:zoomed}. We also show all of our generated results on text-to-3d and image-to-3d tasks in Fig.~\ref{fig:all_results}
Note that we also generate our results and comparison in the videos. Please see our generated video format.

% 

% Having the supplementary compiled together with the main paper means that:
% % 
% \begin{itemize}
% \item The supplementary can back-reference sections of the main paper, for example, we can refer to \cref{sec:intro};
% \item The main paper can forward reference sub-sections within the supplementary explicitly (e.g. referring to a particular experiment); 
% \item When submitted to arXiv, the supplementary will already included at the end of the paper.
% \end{itemize}
% % 
% To split the supplementary pages from the main paper, you can use \href{https://support.apple.com/en-ca/guide/preview/prvw11793/mac#:~:text=Delete%20a%20page%20from%20a,or%20choose%20Edit%20%3E%20Delete).}{Preview (on macOS)}, \href{https://www.adobe.com/acrobat/how-to/delete-pages-from-pdf.html#:~:text=Choose%20%E2%80%9CTools%E2%80%9D%20%3E%20%E2%80%9COrganize,or%20pages%20from%20the%20file.}{Adobe Acrobat} (on all OSs), as well as \href{https://superuser.com/questions/517986/is-it-possible-to-delete-some-pages-of-a-pdf-document}{command line tools}.
